# Supplementary material for: PCB-RandNet: Rethinking Random Sampling for LIDAR Semantic Segmentation in Autonomous Driving Scene
Source: arXiv:2209.13797 source file (2024-03-06)
Supplement: Supplementary file 1 [file appendix.pdf]

# Supplementary Material

## A Limitation and Future Work

### Limitation of PCB-RS

PCB-RS may have the following problems:

- During the algorithmic flow of PCB-RS, since the cylindrical blocks and the number of points in each block shows a long-tailed distribution, taking out a certain number of points from different cylindrical blocks can be considered a typical long-tailed distribution problem. We used a strategy of forced balancing (i.e. balancing the number of points per block so that they are as equal as possible) to deal with this problem. However, whether there is a better way to deal with this problem is our further future work.
- We implement the PCB-RS method based on vanilla Python and Numpy, so in the ablation experiments section of the main text, we compare the RS and FPS sampling methods implemented in the same way. For the RS method, this comparison is fair. Because in RandLA-Net [Hu et al. 2020], it's also implemented using NumPy. However, the FPS method can achieve faster speeds with an efficient CUDA implementation. Therefore, the comparison with FPS is “*potentially unfair*”. Faster implementations of PCB-RS (e.g. CUDA, Numba) will also be seen as further work.

### Limitation of SCL

The main limitation of Sampling Consistency Loss comes from the larger GPU memory consumption and longer training time. However, as shown by the dashed line in the network structure figure in main text, our Sampling Consistency Loss is only utilized during training and discarded during inference, i.e., it is disposable. Therefore, it does not introduce any computational burden during inference.

### Limitation of our method

Since we only study the effect of the sampling method in this paper, we do not make any adjustments to the baseline network structure [Hu et al. 2020, Shuai, Xu, and Liu 2021, Qiu, Anwar, and Barnes 2021]. However, the point cloud distributions under RS and PCB-RS sampling methods are very different. Therefore it is necessary to design more suitable local feature extraction and local feature aggregation operators for PCB-RS sampling. This will be considered as our future work.

## B More visualization and statistical analysis comparisons between RS and PCB-RS

Figure 2 shows more examples of comparisons between RS and PCB-RS similar to those in the main text. These visualizations show that PCB-RS can change the point distribution with respect to distance to sensor by retaining the points at medium and long distances.

## C Ablation studies about Resolution of Polar Cylinder

Ablation studies about resolution of the polar cylinder representation are reported in Table 1. The results show that PCB-RS is relatively robust to the size setting of the resolution of polar cylinder.

Table 1: Effect of of Resolution of Polar Cylinder on SemanticKITTI validation set.

| Resolution of Polar Cylinder | None (Baseline with RS) | $32 \times 32 \times 16$ | $48 \times 48 \times 16$ | $64 \times 64 \times 16$ | $96 \times 96 \times 32$ |
|------------------------------|-------------------------|--------------------------|--------------------------|--------------------------|--------------------------|
| mIoU(%)                      | 52.02                   | 54.34                    | 54.67                    | <b>55.04</b>             | 53.46                    |

## D Qualitative results comparison on SemanticKITTI validation set

Figure 2 shows qualitative visualization of the segmentation results of our method compared to the baseline on the SemanticKITTI validation set. Compared to the baseline, our method has fewer false predictions, while the improvement is more significant at medium and long distances.

## E Quantitative results comparison on SemanticPOSS dataset

The visualization analysis in Figure 3 shows that our method achieves better segmentation performance at different baselines for different distance ranges on SemanticPOSS dataset, which is precisely the result expected from our new PCB-RS sampling method and SCL loss. Table 2, 3, 4 further list the segmentation performance improvement of our proposed method for different distance ranges when RandLA-Net [Hu et al. 2020], BAAF [Qiu, Anwar, and Barnes 2021], BAF-LAC [Shuai, Xu, and Liu 2021] is used as the baseline.

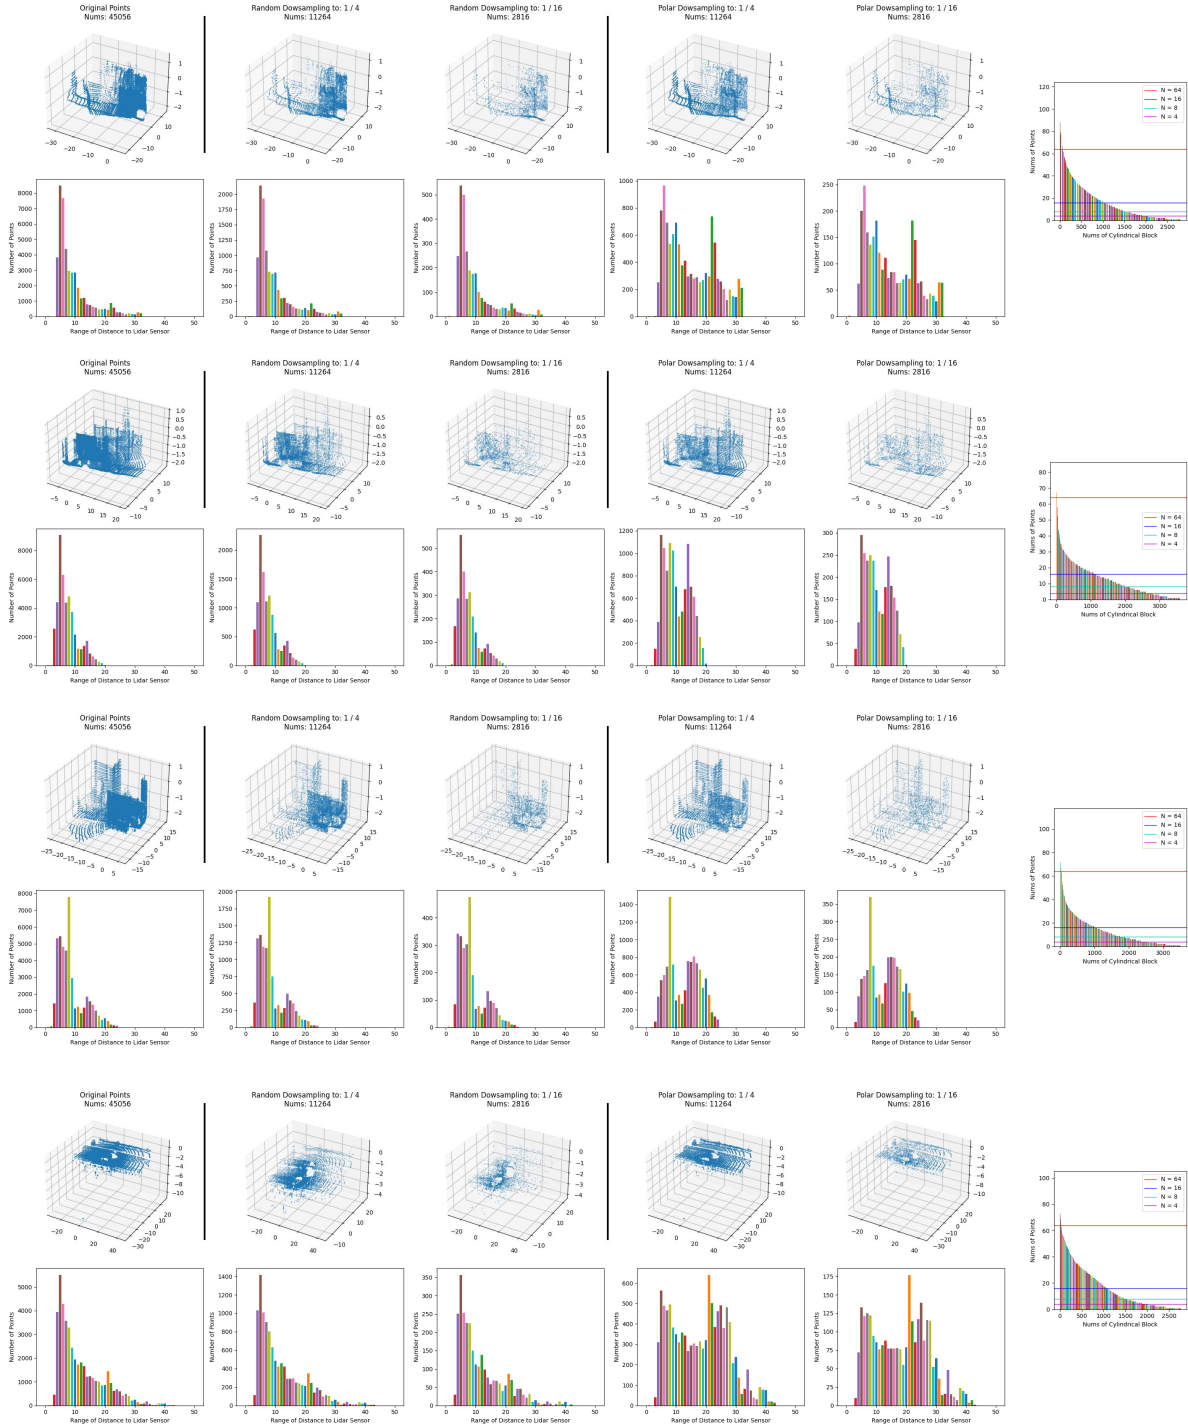

Figure 1: Comparison of qualitative visualization and quantitative statistical analysis between RS and PCB-RS. In each subcase, the upper part shows the visualization of the point cloud, and the lower part shows the distribution of that point cloud at different distance ranges. The subplot on the right shows the distribution of the number of points within the cylindrical block when using the PCB-RS method. *Best viewed in color and zoomed in for more detail.*

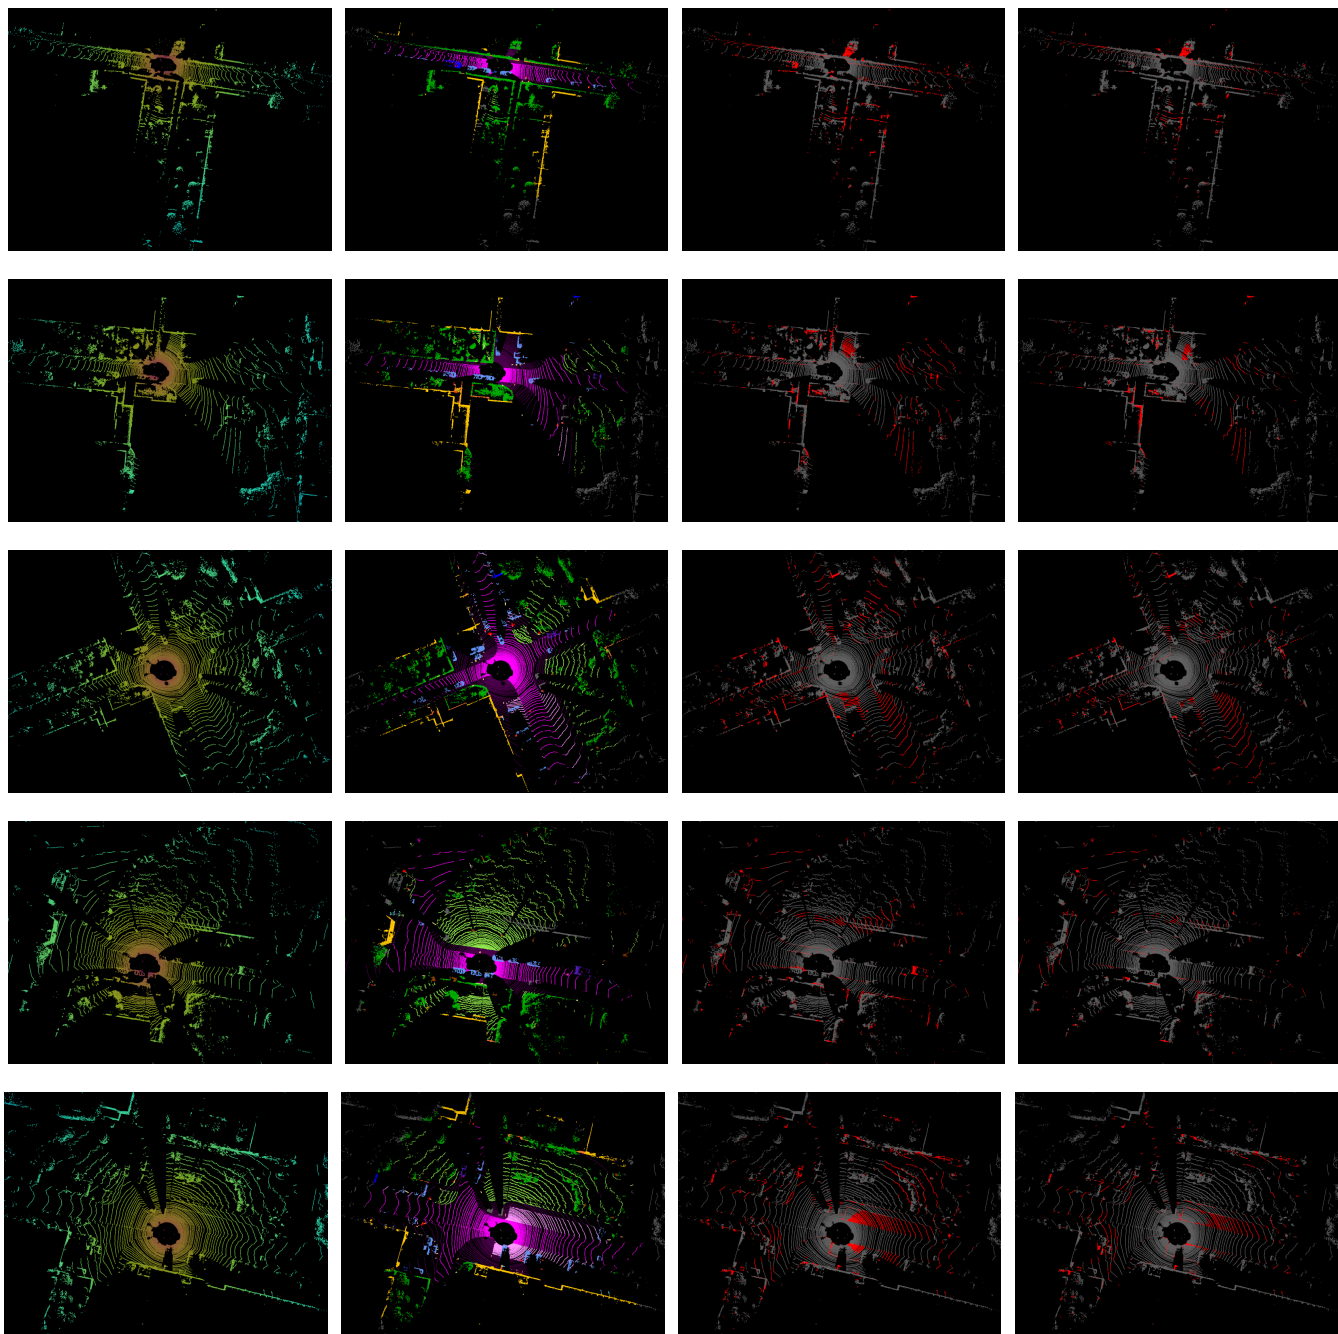

(a) Input Point Cloud

(b) Ground Truth

(c) RandLA-Net

(d) PCB-RandNet

Figure 2: Qualitative analysis on SemanticKITTI validation set. Where (a) and (b) are input data of the LIDAR scan frame and corresponding segmentation ground truth, (c) and (d) are segmentation error maps in this scan frame for baseline and our method. (With red indicating wrong prediction)

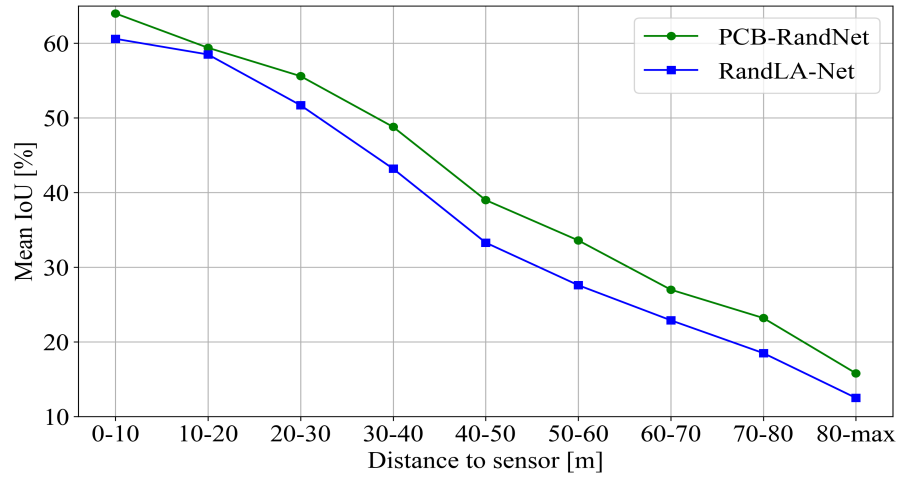

(a) Baseline: RandLA-Net [Hu et al. 2020]

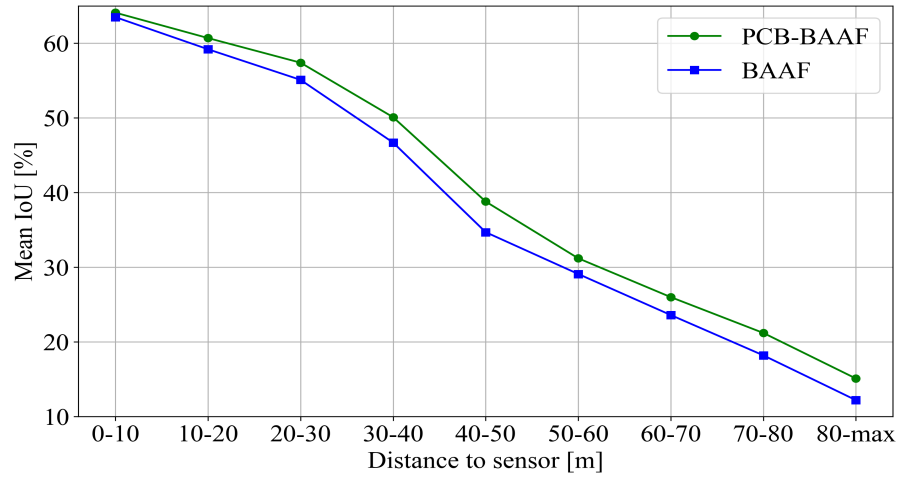

(b) Baseline: BAAF [Qiu, Anwar, and Barnes 2021]

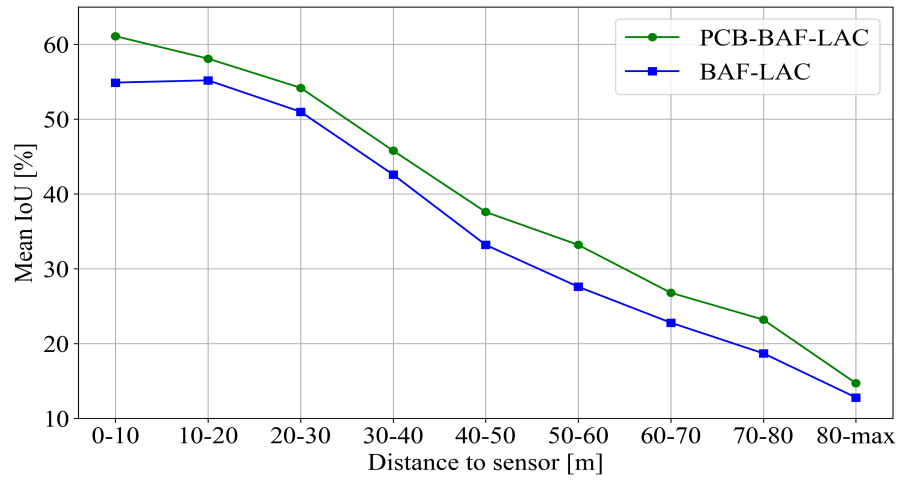

(c) Baseline: BAF-LAC [Shuai, Xu, and Liu 2021]

Figure 3: Evaluation of segmentation performance at different distance ranges on SemanticPOSS with different baselines.

Table 2: Evaluation results on the SemanticPOSS dataset with RandLA-Net as baseline.

|                         | person       | rider        | car          | trunk        | plants       | traffic sign | pole         | building     | fence        | bike         | road         | mIoU         |
|-------------------------|--------------|--------------|--------------|--------------|--------------|--------------|--------------|--------------|--------------|--------------|--------------|--------------|
| Range From 0 m to 10 m  | 74.3<br>68.4 | 63.8<br>56.7 | 62.5<br>92.5 | 46.1<br>50.9 | 75.0<br>80.0 | 21.6<br>32.5 | 44.2<br>27.4 | 61.9<br>77.0 | 78.1<br>75.3 | 46.5<br>50.3 | 92.1<br>93.3 | 60.6<br>64.0 |
| Improvement             | -5.9         | -7.1         | 30.0         | 4.8          | 5.0          | 10.9         | -16.8        | 15.1         | -2.8         | 3.8          | 1.2          | 3.4          |
| Range From 10 m to 20 m | 72.2<br>65.6 | 62.5<br>54.5 | 62.3<br>65.7 | 33.7<br>38.0 | 78.8<br>82.2 | 24.5<br>33.8 | 40.6<br>34.0 | 70.5<br>78.1 | 54.8<br>52.2 | 57.3<br>61.9 | 85.9<br>87.8 | 58.5<br>59.4 |
| Improvement             | -6.6         | -8.0         | 3.4          | 4.3          | 3.4          | 9.3          | -6.6         | 7.6          | -2.6         | 4.6          | 1.9          | 0.9          |
| Range From 20 m to 30 m | 64.3<br>63.7 | 54.6<br>52.9 | 47.8<br>56.1 | 30.8<br>33.0 | 73.0<br>77.3 | 24.2<br>31.5 | 39.2<br>40.3 | 81.8<br>84.5 | 33.3<br>41.5 | 47.3<br>50.9 | 72.2<br>80.4 | 51.7<br>55.6 |
| Improvement             | -0.6         | -1.7         | 8.3          | 2.2          | 4.3          | 7.3          | 1.1          | 2.7          | 8.2          | 3.6          | 8.2          | 3.9          |
| Range From 30 m to 40 m | 38.7<br>40.7 | 35.3<br>36.3 | 41.2<br>55.7 | 23.3<br>24.6 | 69.7<br>75.4 | 26.4<br>29.0 | 41.9<br>54.8 | 81.1<br>83.6 | 19.0<br>26.2 | 32.7<br>35.9 | 65.6<br>74.2 | 43.2<br>48.8 |
| Improvement             | 2.0          | 1.0          | 14.5         | 1.3          | 5.7          | 2.6          | 12.9         | 2.5          | 7.2          | 3.2          | 8.6          | 5.6          |
| Range From 40 m to 50 m | 20.5<br>25.2 | 16.8<br>18.0 | 28.0<br>36.1 | 19.9<br>17.1 | 63.9<br>72.2 | 19.0<br>21.8 | 25.0<br>41.8 | 76.1<br>80.3 | 11.9<br>17.3 | 25.5<br>32.2 | 59.8<br>67.2 | 33.3<br>39.0 |
| Improvement             | 4.7          | 1.2          | 8.1          | -2.8         | 8.3          | 2.8          | 16.8         | 4.2          | 5.4          | 6.7          | 7.4          | 5.7          |
| Range From 50 m to 60 m | 17.6<br>22.1 | 2.7<br>1.4   | 23.1<br>36.8 | 10.4<br>13.5 | 61.3<br>69.7 | 17.2<br>18.1 | 19.8<br>36.6 | 78.7<br>83.3 | 7.6<br>11.2  | 17.6<br>24.3 | 47.5<br>52.8 | 27.6<br>33.6 |
| Improvement             | 4.5          | -1.3         | 13.7         | 3.1          | 8.4          | 0.9          | 16.8         | 4.6          | 3.6          | 6.7          | 5.3          | 6.0          |
| Range From 60 m to 70 m | 13.6<br>16.6 | 0.3<br>0.0   | 5.6<br>8.5   | 6.0<br>8.8   | 65.0<br>71.9 | 11.9<br>19.0 | 15.5<br>24.8 | 78.3<br>82.9 | 13.5<br>16.3 | 14.9<br>15.8 | 27.5<br>32.3 | 22.9<br>27.0 |
| Improvement             | 3.0          | -0.3         | 2.9          | 2.8          | 6.9          | 7.1          | 9.3          | 4.6          | 2.8          | 0.9          | 4.8          | 4.1          |
| Range From 70 m to 80 m | 8.2<br>15.3  | 0.0<br>0.0   | 2.0<br>4.2   | 5.4<br>4.1   | 58.1<br>70.5 | 3.3<br>12.4  | 13.4<br>23.9 | 79.0<br>84.6 | 4.4<br>11.5  | 7.4<br>6.3   | 21.8<br>22.2 | 18.5<br>23.2 |
| Improvement             | 7.1          | 0.0          | 2.2          | -1.3         | 12.4         | 9.1          | 10.5         | 5.6          | 7.1          | -1.1         | 0.4          | 4.7          |
| Range Above 80 m        | 2.0<br>4.9   | 0.0<br>0.0   | 0.4<br>0.5   | 4.9<br>3.2   | 35.9<br>47.5 | 0.6<br>0.7   | 4.8<br>15.8  | 63.6<br>74.9 | 1.7<br>3.5   | 5.6<br>3.2   | 18.0<br>19.4 | 12.5<br>15.8 |
| Improvement             | 2.9          | 0.0          | 0.1          | -1.7         | 11.6         | 0.1          | 11.0         | 11.3         | 1.8          | -2.4         | 1.4          | 3.3          |
| Total Range             | 56.8<br>57.7 | 58.2<br>52.4 | 48.1<br>61.4 | 37.8<br>42.0 | 73.4<br>78.1 | 22.3<br>31.8 | 35.4<br>33.0 | 76.6<br>81.6 | 45.4<br>51.5 | 45.7<br>51.2 | 80.9<br>84.3 | 52.8<br>56.8 |
| Improvement             | 0.9          | -5.8         | 13.3         | 4.2          | 4.7          | 9.5          | -2.4         | 5.0          | 6.1          | 5.5          | 3.4          | 4.0          |

Table 3: Evaluation results on the SemanticPOSS dataset with BAAF as baseline.

|                         | person | rider | car  | trunk | plants | traffic sign | pole  | building | fence | bike | road | mIoU |
|-------------------------|--------|-------|------|-------|--------|--------------|-------|----------|-------|------|------|------|
| Range From 0 m to 10 m  | 73.0   | 55.2  | 66.3 | 52.3  | 79.3   | 30.5         | 43.1  | 75.1     | 79.7  | 53.3 | 90.6 | 63.5 |
|                         | 70.0   | 58.6  | 88.5 | 52.6  | 81.4   | 34.6         | 30.5  | 60.9     | 79.9  | 54.9 | 92.9 | 64.1 |
| Improvement             | -3.0   | 3.4   | 22.2 | 0.3   | 2.1    | 4.1          | -12.6 | -14.2    | 0.2   | 1.6  | 2.3  | 0.6  |
| Range From 10 m to 20 m | 68.6   | 58.1  | 61.9 | 40.5  | 80.6   | 27.3         | 33.8  | 76.6     | 58.1  | 59.7 | 86.1 | 59.2 |
|                         | 69.6   | 63.6  | 66.1 | 36.2  | 81.7   | 24.6         | 36.3  | 75.4     | 63.7  | 62.6 | 87.8 | 60.7 |
| Improvement             | 1.0    | 5.5   | 4.2  | -4.3  | 1.1    | -2.7         | 2.5   | -1.2     | 5.6   | 2.9  | 1.7  | 1.5  |
| Range From 20 m to 30 m | 64.8   | 54.6  | 55.3 | 35.4  | 76.5   | 26.0         | 39.7  | 84.6     | 39.8  | 49.8 | 79.2 | 55.1 |
|                         | 67.0   | 61.1  | 60.2 | 34.0  | 77.5   | 18.6         | 45.8  | 83.3     | 48.5  | 53.7 | 82.0 | 57.4 |
| Improvement             | 2.2    | 6.5   | 4.9  | -1.4  | 1.0    | -7.4         | 6.1   | -1.3     | 8.7   | 3.9  | 2.8  | 2.3  |
| Range From 30 m to 40 m | 45.1   | 39.6  | 48.1 | 25.8  | 73.5   | 25.1         | 40.8  | 82.6     | 23.7  | 34.0 | 75.7 | 46.7 |
|                         | 43.4   | 43.7  | 57.7 | 24.8  | 75.9   | 27.1         | 49.3  | 83.5     | 31.0  | 38.3 | 76.6 | 50.1 |
| Improvement             | -1.7   | 4.1   | 9.6  | -1.0  | 2.4    | 2.0          | 8.5   | 0.9      | 7.3   | 4.3  | 0.9  | 3.4  |
| Range From 40 m to 50 m | 22.8   | 24.1  | 31.2 | 16.5  | 65.9   | 11.7         | 23.7  | 76.1     | 15.3  | 24.0 | 70.8 | 34.7 |
|                         | 21.7   | 24.7  | 39.5 | 14.1  | 70.6   | 21.1         | 34.1  | 78.8     | 21.6  | 31.1 | 69.9 | 38.8 |
| Improvement             | -1.1   | 0.6   | 8.3  | -2.4  | 4.7    | 9.4          | 10.4  | 2.7      | 6.3   | 7.1  | -0.9 | 4.1  |
| Range From 50 m to 60 m | 19.9   | 10.0  | 24.2 | 13.5  | 60.6   | 10.8         | 21.4  | 79.6     | 8.2   | 16.6 | 55.2 | 29.1 |
|                         | 18.6   | 6.5   | 20.8 | 8.5   | 65.8   | 21.3         | 26.6  | 81.6     | 13.7  | 24.4 | 55.8 | 31.2 |
| Improvement             | -1.3   | -3.5  | -3.4 | -5.0  | 5.2    | 10.5         | 5.2   | 2.0      | 5.5   | 7.8  | 0.6  | 2.1  |
| Range From 60 m to 70 m | 17.6   | 5.2   | 8.0  | 7.6   | 58.2   | 11.8         | 21.9  | 77.9     | 9.3   | 10.4 | 32.2 | 23.6 |
|                         | 16.8   | 0.5   | 7.4  | 11.7  | 66.9   | 7.4          | 20.8  | 81.6     | 22.1  | 17.4 | 33.0 | 26.0 |
| Improvement             | -0.8   | -4.7  | -0.6 | 4.1   | 8.7    | -4.4         | -1.1  | 3.7      | 12.8  | 7.0  | 0.8  | 2.4  |
| Range From 70 m to 80 m | 9.5    | 0.1   | 4.9  | 1.7   | 49.4   | 7.1          | 18.7  | 74.8     | 6.7   | 6.4  | 20.6 | 18.2 |
|                         | 11.3   | 0.0   | 3.7  | 8.3   | 64.6   | 3.7          | 17.9  | 82.5     | 10.3  | 9.7  | 21.3 | 21.2 |
| Improvement             | 1.8    | -0.1  | -1.2 | 6.6   | 15.2   | -3.4         | -0.8  | 7.7      | 3.6   | 3.3  | 0.7  | 3.0  |
| Range Above 80 m        | 2.6    | 0.0   | 1.2  | 5.1   | 29.3   | 0.7          | 11.6  | 66.5     | 2.1   | 4.2  | 10.6 | 12.2 |
|                         | 3.7    | 0.0   | 1.8  | 6.4   | 44.6   | 0.2          | 8.8   | 73.3     | 3.9   | 4.7  | 19.2 | 15.1 |
| Improvement             | 1.1    | 0.0   | 0.6  | 1.3   | 15.3   | -0.5         | -2.8  | 6.8      | 1.8   | 0.5  | 8.6  | 2.9  |
| Total Range             | 57.5   | 53.1  | 51.7 | 42.4  | 75.7   | 26.7         | 36.5  | 79.5     | 51.4  | 47.4 | 83.4 | 55.0 |
|                         | 58.1   | 57.6  | 63.2 | 41.8  | 77.9   | 28.9         | 33.8  | 79.8     | 60.1  | 52.2 | 84.9 | 58.0 |
| Improvement             | 0.6    | 4.5   | 11.5 | -0.6  | 2.2    | 2.2          | -2.7  | 0.3      | 8.7   | 4.8  | 1.5  | 3.0  |

Table 4: Evaluation results on the SemanticPOSS dataset with BAF-LAC as baseline.

|                         | person | rider | car   | trunk | plants | traffic sign | pole | building | fence | bike | road | mIoU |
|-------------------------|--------|-------|-------|-------|--------|--------------|------|----------|-------|------|------|------|
| Range From 0 m to 10 m  | 66.7   | 49.0  | 78.8  | 54.1  | 73.7   | 26.1         | 32.5 | 12.5     | 68.6  | 51.3 | 91.2 | 54.9 |
|                         | 66.9   | 63.0  | 89.3  | 54.2  | 78.1   | 33.5         | 55.1 | 2.9      | 78.9  | 58.1 | 92.2 | 61.1 |
| Improvement             | 0.2    | 14.0  | 10.5  | 0.1   | 4.4    | 7.4          | 22.6 | -9.6     | 10.3  | 6.8  | 1.0  | 6.2  |
| Range From 10 m to 20 m | 66.9   | 54.1  | 64.9  | 34.3  | 77.6   | 21.7         | 28.8 | 64.2     | 48.3  | 59.5 | 86.7 | 55.2 |
|                         | 68.0   | 58.0  | 62.8  | 42.6  | 75.7   | 32.0         | 39.0 | 59.0     | 54.1  | 61.1 | 86.5 | 58.1 |
| Improvement             | 1.1    | 3.9   | -2.1  | 8.3   | -1.9   | 10.3         | 10.2 | -5.2     | 5.8   | 1.6  | -0.2 | 2.9  |
| Range From 20 m to 30 m | 59.7   | 54.4  | 52.9  | 32.3  | 72.7   | 14.9         | 38.7 | 81.5     | 31.0  | 50.5 | 73.1 | 51.0 |
|                         | 59.0   | 55.8  | 47.7  | 35.8  | 73.3   | 32.0         | 41.6 | 79.0     | 41.4  | 49.7 | 80.6 | 54.2 |
| Improvement             | -0.7   | 1.4   | -5.2  | 3.5   | 0.6    | 17.1         | 2.9  | -2.5     | 10.4  | -0.8 | 7.5  | 3.2  |
| Range From 30 m to 40 m | 35.0   | 34.7  | 46.4  | 27.1  | 69.2   | 19.2         | 43.9 | 80.8     | 16.6  | 33.1 | 62.3 | 42.6 |
|                         | 36.5   | 43.7  | 36.3  | 27.5  | 73.2   | 28.9         | 41.3 | 80.4     | 24.8  | 35.0 | 76.2 | 45.8 |
| Improvement             | 1.5    | 9.0   | -10.1 | 0.4   | 4.0    | 9.7          | -2.6 | -0.4     | 8.2   | 1.9  | 13.9 | 3.2  |
| Range From 40 m to 50 m | 16.8   | 20.4  | 35.2  | 14.4  | 63.4   | 17.6         | 23.6 | 76.9     | 12.9  | 26.2 | 57.4 | 33.2 |
|                         | 20.1   | 34.7  | 22.5  | 19.2  | 70.1   | 24.0         | 27.8 | 78.7     | 16.6  | 29.2 | 71.0 | 37.6 |
| Improvement             | 3.3    | 14.3  | -12.7 | 4.8   | 6.7    | 6.4          | 4.2  | 1.8      | 3.7   | 3.0  | 13.6 | 4.4  |
| Range From 50 m to 60 m | 14.1   | 1.2   | 23.7  | 5.7   | 61.8   | 25.5         | 17.8 | 81.1     | 8.0   | 20.4 | 44.4 | 27.6 |
|                         | 20.7   | 7.1   | 19.6  | 12.3  | 67.7   | 31.9         | 30.1 | 82.2     | 12.0  | 24.5 | 57.2 | 33.2 |
| Improvement             | 6.6    | 5.9   | -4.1  | 6.6   | 5.9    | 6.4          | 12.3 | 1.1      | 4.0   | 4.1  | 12.8 | 5.6  |
| Range From 60 m to 70 m | 14.1   | 0.3   | 10.6  | 4.0   | 61.6   | 17.3         | 14.5 | 79.6     | 8.3   | 16.9 | 23.5 | 22.8 |
|                         | 18.1   | 0.2   | 6.5   | 6.3   | 68.5   | 27.0         | 22.5 | 81.1     | 13.2  | 17.1 | 34.5 | 26.8 |
| Improvement             | 4.0    | -0.1  | -4.1  | 2.3   | 6.9    | 9.7          | 8.0  | 1.5      | 4.9   | 0.2  | 11.0 | 4.0  |
| Range From 70 m to 80 m | 9.9    | 0.0   | 3.7   | 3.5   | 55.6   | 9.6          | 11.6 | 79.7     | 6.6   | 8.3  | 16.6 | 18.7 |
|                         | 16.4   | 0.0   | 3.3   | 5.6   | 64.6   | 26.6         | 20.9 | 80.9     | 6.3   | 8.2  | 22.5 | 23.2 |
| Improvement             | 6.5    | 0.0   | -0.4  | 2.1   | 9.0    | 17.0         | 9.3  | 1.2      | -0.3  | -0.1 | 5.9  | 4.5  |
| Range Above 80 m        | 3.7    | 0.0   | 0.8   | 4.5   | 34.6   | 3.4          | 4.8  | 70.1     | 3.5   | 4.4  | 10.6 | 12.8 |
|                         | 6.2    | 0.0   | 0.1   | 3.4   | 41.2   | 3.5          | 11.1 | 72.0     | 0.1   | 2.6  | 21.5 | 14.7 |
| Improvement             | 2.5    | 0.0   | -0.7  | -1.1  | 6.6    | 0.1          | 6.3  | 1.9      | -3.4  | -1.8 | 10.9 | 1.9  |
| Total Range             | 50.4   | 48.7  | 54.4  | 40.0  | 72.5   | 22.4         | 28.1 | 74.5     | 42.0  | 48.8 | 81.0 | 51.2 |
|                         | 56.4   | 57.7  | 53.8  | 43.5  | 73.9   | 32.1         | 43.3 | 72.5     | 52.8  | 51.4 | 83.8 | 56.5 |
| Improvement             | 6.0    | 9.0   | -0.6  | 3.5   | 1.4    | 9.7          | 15.2 | -2.0     | 10.8  | 2.6  | 2.8  | 5.3  |

## References

- Hu, Q.; Yang, B.; Xie, L.; Rosa, S.; Guo, Y.; Wang, Z.; Trigoni, N.; and Markham, A. 2020. Randla-net: Efficient semantic segmentation of large-scale point clouds. In *CVPR*, 11108–11117. 1, 4
- Qiu, S.; Anwar, S.; and Barnes, N. 2021. Semantic segmentation for real point cloud scenes via bilateral augmentation and adaptive fusion. In *CVPR*, 1757–1767. 1, 4
- Shuai, H.; Xu, X.; and Liu, Q. 2021. Backward Attentive Fusing Network With Local Aggregation Classifier for 3D Point Cloud Semantic Segmentation. *IEEE Transactions on Image Processing*, 30: 4973–4984. 1, 4
